# Supplementary material for: Impact of solvent on state-to-state population transport in multistate systems using coherences
Source: arXiv:2301.12712 ancillary file (2023-02-24)
Supplement: Supplementary file 1 [file supp_info.pdf]

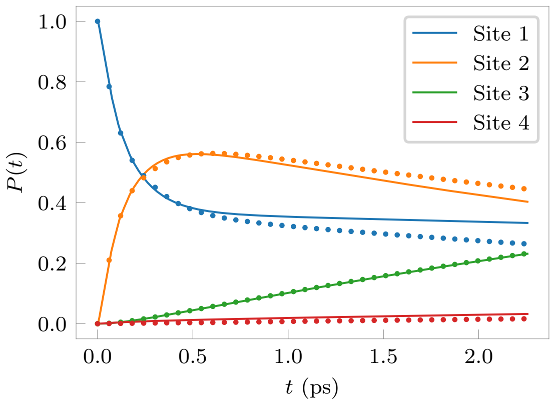


FIG. 1. Comparison of the dynamics of the full FMO vis-a-vis the coarse-grained 4-site model.

## I. SYSTEM HAMILTONIAN

The following is the system Hamiltonian for the reduced 4-site FMO model:

$$H = \begin{pmatrix} 168.68 & -92.21 & 3.58 & -9.79 \\ -92.21 & 47.26 & 18.99 & 7.13 \\ 3.58 & 18.99 & -612.21 & -45.60 \\ -9.79 & 7.13 & -45.60 & 21.27 \end{pmatrix} \text{cm}^{-1} \tag{1}$$

Figure 1 shows a comparison between the dynamics of the first four sites for the full FMO versus the coarse-grained model. One can see the similar dynamics and timescales in both.

## II. EFFECT OF SCALING OF REORGANIZATION ENERGY ON THE EXCITONIC POPULATION ON VARIOUS SITES

We report the time-dependent populations of each of the BChl sites on scanning across the reorganization energies on sites 3 and 2 in Figs. 2 and 3 respectively. In Fig. 3, notice that scanning the reorganization energy on site 3 has very minimal effect on the population of site 1. The effect is much more observable for the populations of site 2 onwards. However, on changing the reorganization energy on site 2 (Fig. 3), the dynamics on all the sites seem to be effected.

On changing the reorganization energy on site 2 (Fig. 3) we see the populations of site 1 and site 2 changing in very non-trivial ways. The total population on site 3 seems to show a behavior similar to that seen while scanning in Fig. 2.

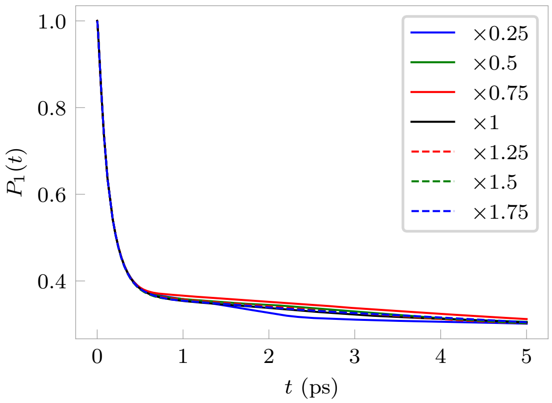


(a) Population of Site 1

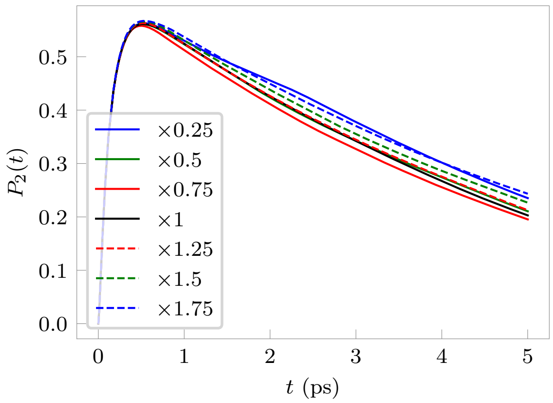


(b) Population of Site 2

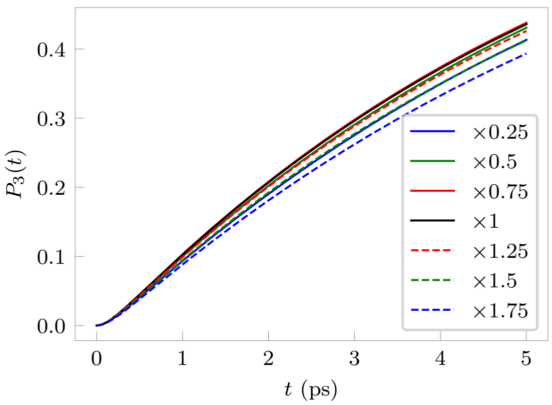


(c) Population of Site 3

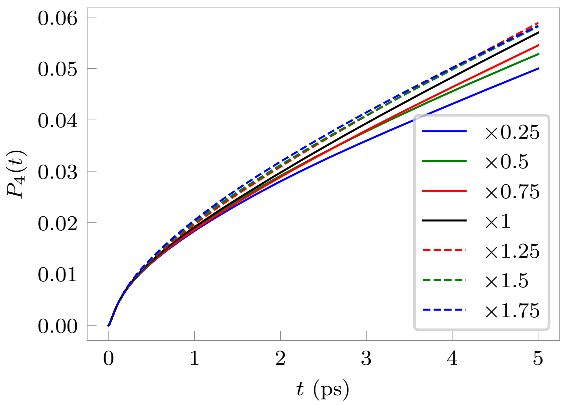


(d) Population of Site 4

FIG. 2. Site-specific population dynamics on scanning across the reorganization energy on site 3.

Additionally, as shown in the body of the paper, one can study the channel dependent population transfer. While we have explored the channels relevant for the two main pathways, $1 \to 2 \to 3$ and $1 \to 4 \to 3$, of exciton transfer in the coarse-grained model, here we plot all the remaining pathways for completeness. In Fig. 4, we show the effect of scanning the reorganization energy on the 3rd site. Figure 5 shows the effect of doing the same on the 2nd site.

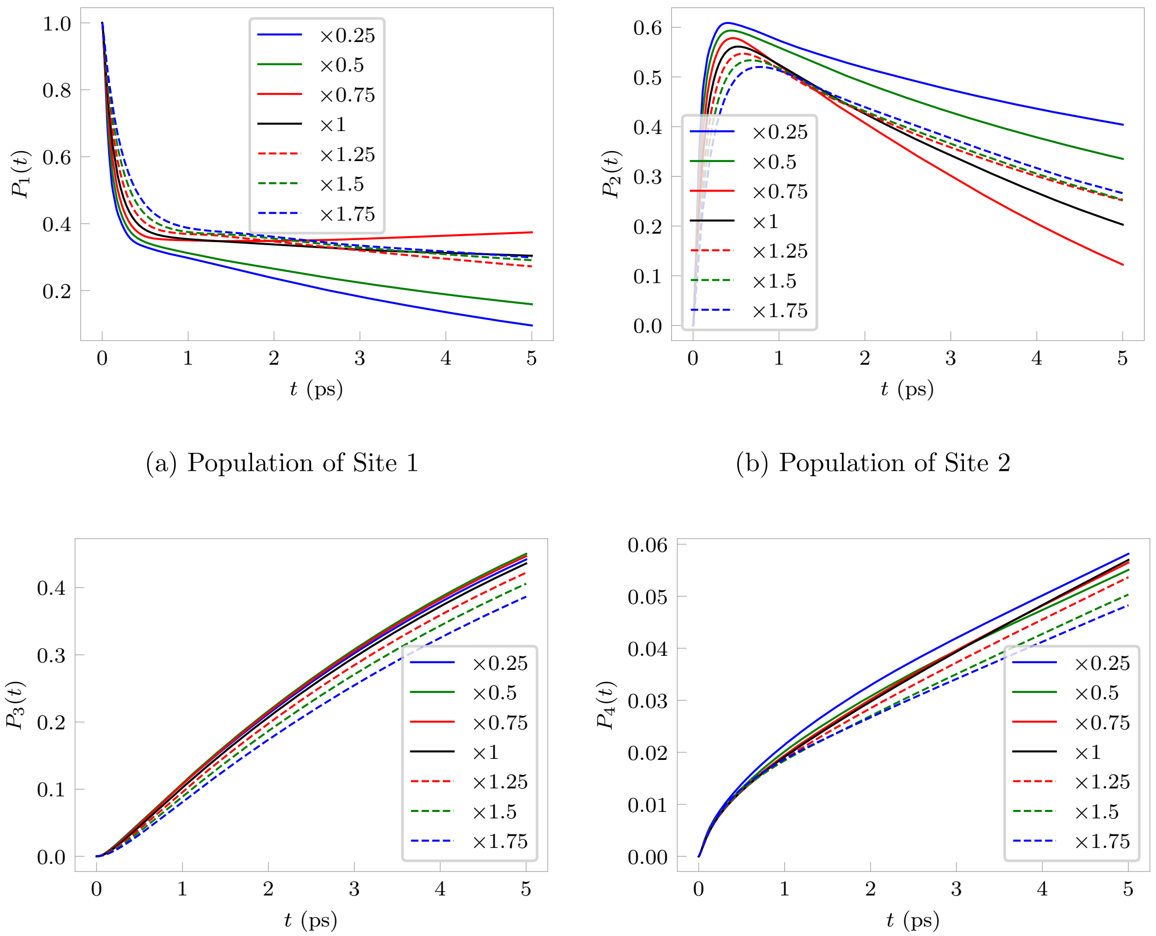


(a) Population of Site 1

(b) Population of Site 2

(c) Population of Site 3

(d) Population of Site 4

FIG. 3. Site-specific population dynamics on scanning across the reorganization energy on site 2.

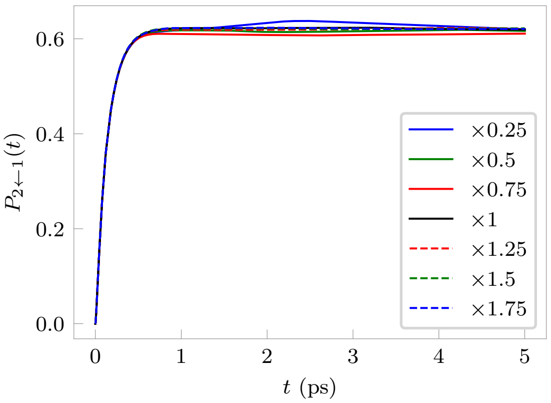


(a) Direct transfer from Site 1 to 2

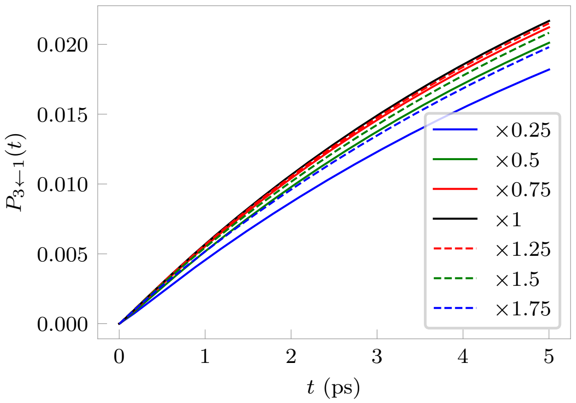


(b) Direct transfer from Site 1 to 3

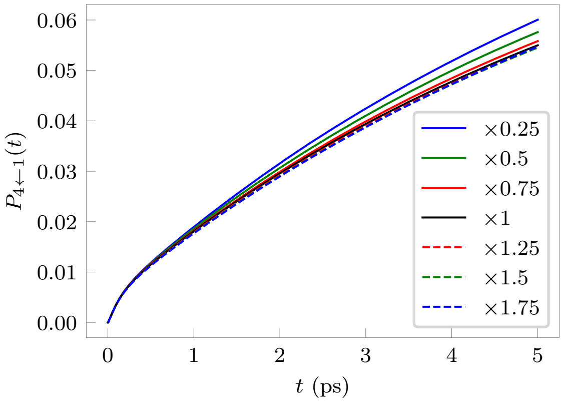


(c) Direct transfer from Site 1 to 4

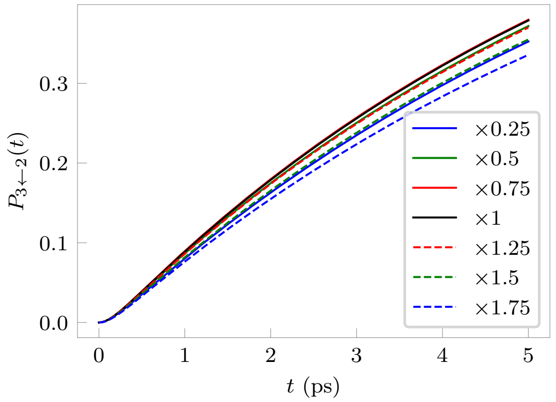


(d) Direct transfer from Site 2 to 3

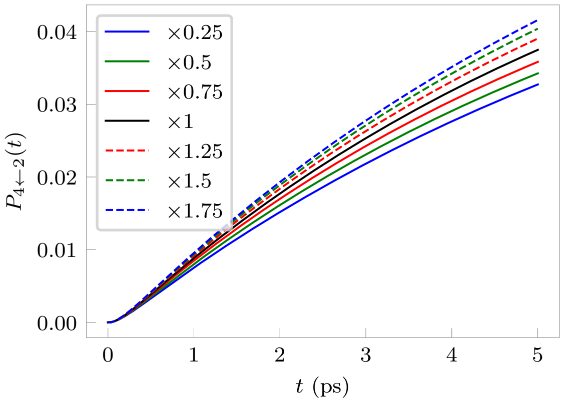


(e) Direct transfer from Site 2 to 4

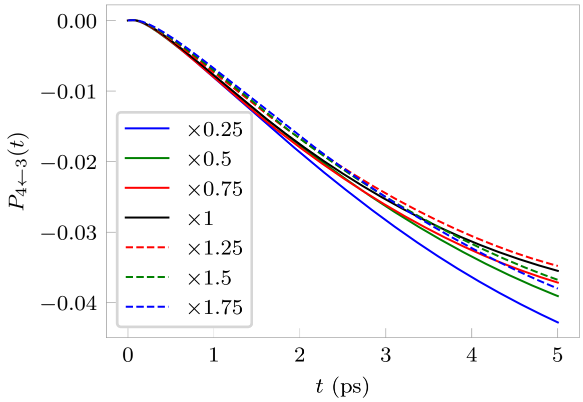


(f) Direct transfer from Site 3 to 4

FIG. 4. Effect of scanning reorganization energy of site 3 on the transfers.

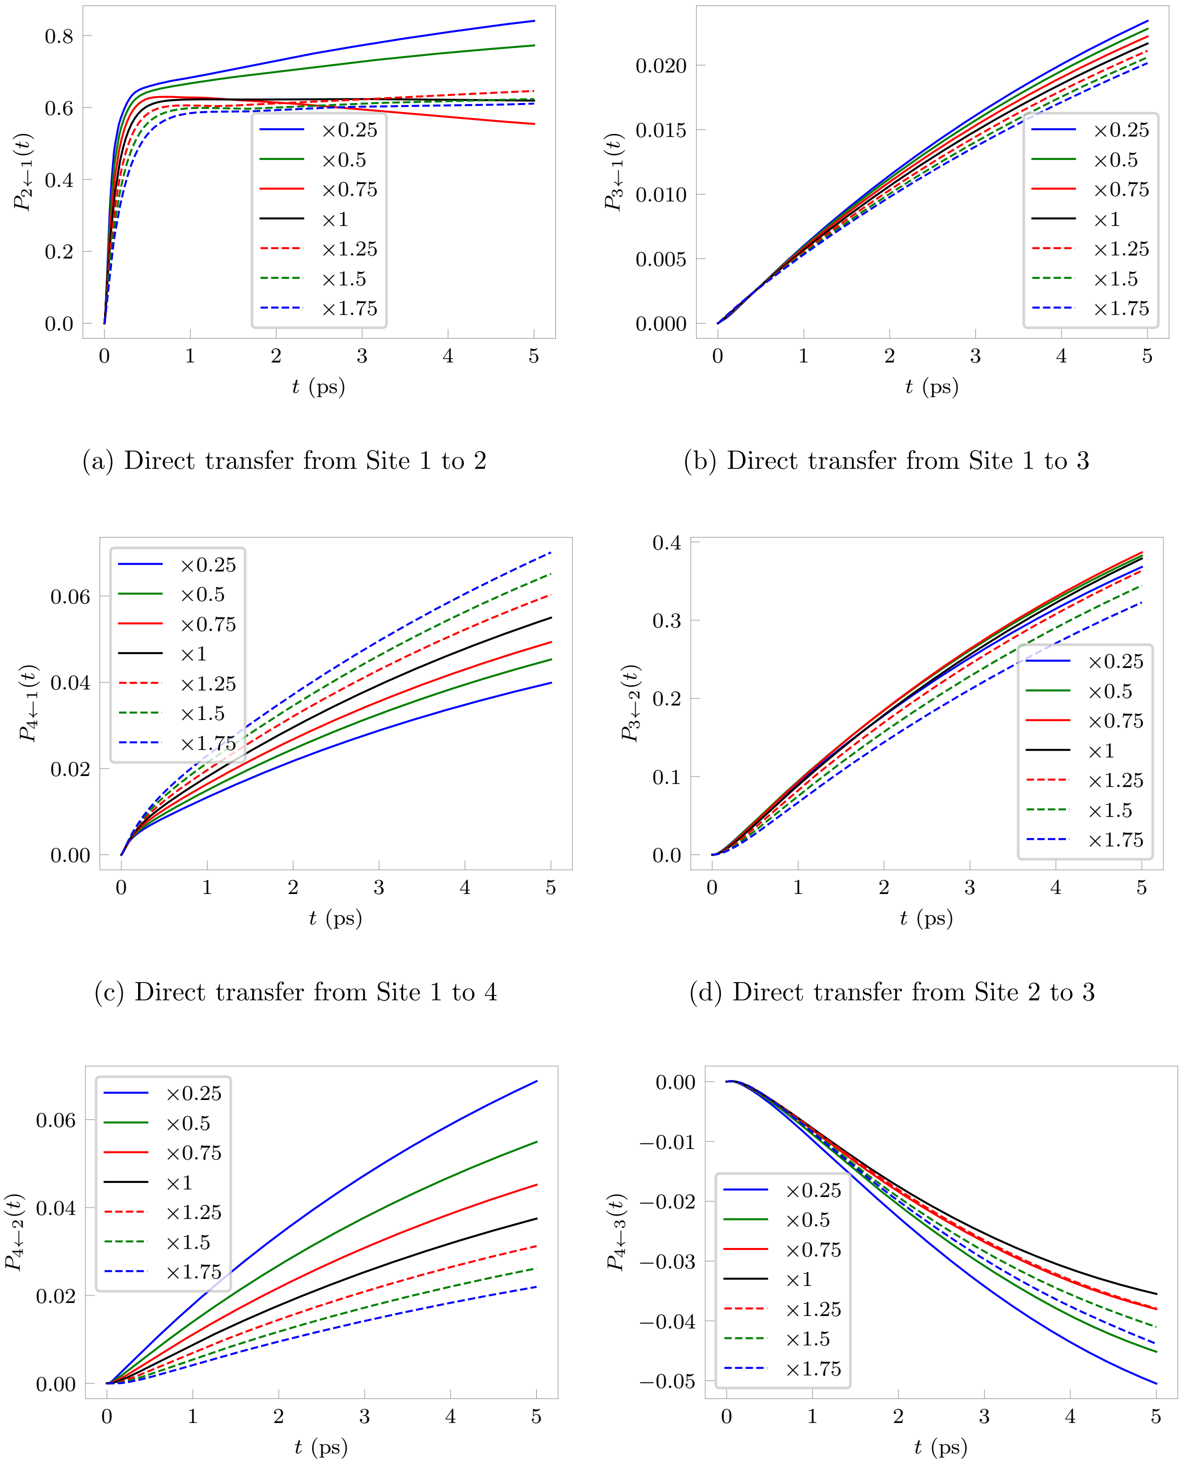


(a) Direct transfer from Site 1 to 2

(b) Direct transfer from Site 1 to 3

(c) Direct transfer from Site 1 to 4

(d) Direct transfer from Site 2 to 3

(e) Direct transfer from Site 2 to 4

(f) Direct transfer from Site 3 to 4

FIG. 5. Effect of scanning reorganization energy of site on the transfers.
